# Supplementary material for: Causal Distillation for Alleviating Performance Heterogeneity in Recommender Systems
Source: arXiv:2405.20626 source file (2024-05-31)
Supplement: Supplementary file 1 [file 6.Appendix.tex]

\section{Appendix}
\label{sec:appendix}
